# Supplementary material for: New Tessellation-Based Procedure to Design Perfectly Hyperuniform Disordered Dispersions for Materials Discovery
Source: arXiv:1901.06037 source file (2019-03-10)
Supplement: Supplementary file 1 [file Supplementary_Materials.pdf]

# Supplementary Materials for
# New Tessellation-Based Procedure to Design Perfectly Hyperuniform Disordered Dispersions


Jaeuk Kim[1] and Salvatore Torquato[1,2,3,4,*]

[1] *Department of Physics, Princeton University, Princeton, New Jersey 08544, USA*
[2] *Department of Chemistry, Princeton University, Princeton, New Jersey 08544, USA*
[3] *Princeton Institute for the Science and Technology of Materials, Princeton University, Princeton, New Jersey 08544, USA*
[4] *Program in Applied and Computational Mathematics, Princeton University, Princeton, New Jersey 08544, USA*



(Dated: November 30, 2018)


## I. VORONOI TESSELLATIONS

We describe how we compute the Voronoi tessellations of a given point pattern in a $d$-dimensional cubic periodic simulation box of side length $L$. To enhance the performance, we divide point patterns into several domains and compute Voronoi tessellation of each domain in parallel. Specifically, we select domains in the following steps (see Fig. 1):

1. Divide the simulation box into disjoint cubic regions of a fixed side length $l$, called subdomains.

2. For each subdomain, make a marginal region that surrounds the subdomain. A subdomain and the associated marginal region comprises a domain. Each domain stores the position coordinates of all points that lie within it. We set thickness of $W = 6\rho^{-1/d}$, where $\rho$ is the number density of the point pattern.

Then, we can compute the Voronoi cells in each subdomain in parallel.

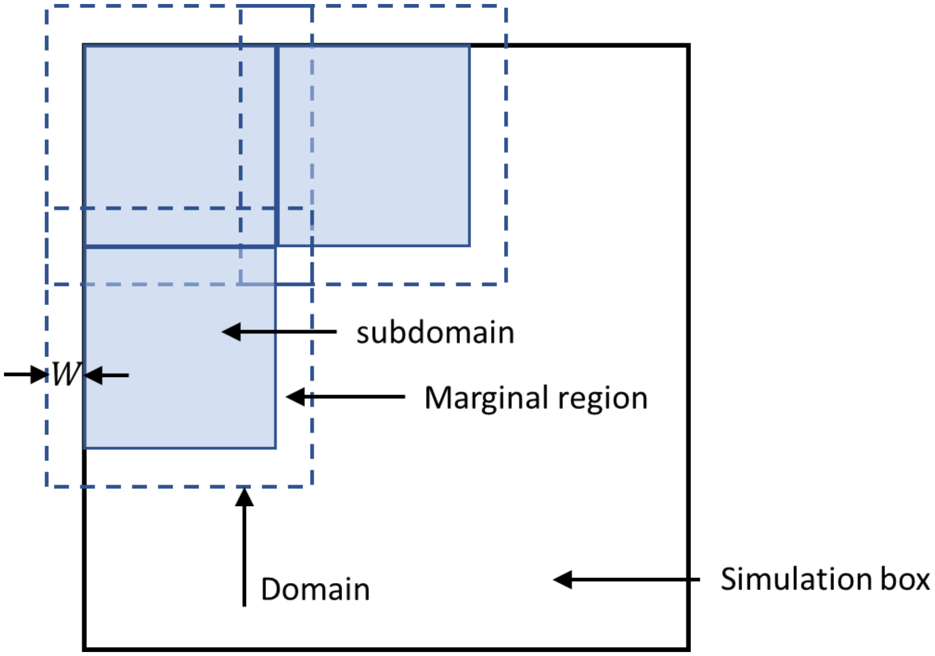


FIG. 1. Schematic of implementation of VORO++ library [1]. A point pattern in a periodic simulation box is sampled by domains of equal size (squares bounded by dashed lines). Each domain consists of a subdomain (a shaded region in center) and a marginal region surrounding the subdomain. Subdomains are mutually disjoint and fully cover a simulation box. Thickness of the marginal region is denoted by $W$.

We should note that the thickness $W$ should not be smaller than the largest hole diameter. Furthermore, in 2D implementation of VORO++, one should judiciously choose the domain size $(2W + l)$ such that the particle number in each domain do not exceed $10^5$.

## II. PROGENITOR PACKINGS FOR VORONOI TESSELLATIONS

Here, we summarize simulation parameters in the progenitor packings (TABLE. I) and some simulation results for the constructed dispersions (TABLE. II).

TABLE I. Progenitor packings used for Voronoi tessellations

| Progenitor packings | Particle number $N$ | The number of packings | Computational time (mins/configs) |
|---|---|---|---|
| 2D saturated RSA | 1.008(8) $\times 10^3$ | 10000 | $\ll 1$ |
| 2D saturated RSA | 1.006(2) $\times 10^4$ | 1000 | 1/100 |
| 2D saturated RSA | 1.0053(7) $\times 10^5$ | 100 | 1/2 |
| 2D saturated RSA | 1.0053(3) $\times 10^6$ | 50 | 43 |
| 2D saturated RSA | 1.00525(8) $\times 10^7$ | 25 | 112 |
| 3D saturated RSA | 1.007(7) $\times 10^3$ | 10000 | $< 1/100$ |
| 3D saturated RSA | 1.004(2) $\times 10^4$ | 1000 | 1/15 |
| 3D saturated RSA | 1.0031(8) $\times 10^5$ | 100 | 1 |
| 3D saturated RSA | 1.0031(2) $\times 10^6$ | 50 | $\sim 14$ |

[a] All the progenitor packings are set to have unit number density. Computational time represents the average time spent to generate a progenitor packing and the constructed dispersion using 10 2.6-GHz CPUs.

TABLE II. Maximal packing fractions $\phi^{(1)}_{\max}$ and spectral densities at the minimal wavenumber of the constructed dispersions.

| Progenitor Packings | $\phi^{(1)}_{\max}$ | $\tilde{\chi}_V(k \to k_{\min})$ | |
|---|---|---|---|
| | | Constructed dispersions | Scaled progenitor packings |
| 2D saturated RSA ($N \approx 10^3$) | 0.418(14) [0.3626] | 4.74(3) $\times 10^{-10}$ | 5.84(3) $\times 10^{-6}$ |
| 2D saturated RSA ($N \approx 10^4$) | 0.395(10) [0.3581] | 1.94(4) $\times 10^{-12}$ | 5.78(7) $\times 10^{-6}$ |
| 2D saturated RSA ($N \approx 10^5$) | 0.380(7) [0.3580] | 4.54(29) $\times 10^{-14}$ | 5.13(25) $\times 10^{-6}$ |
| 2D saturated RSA ($N \approx 10^6$) | 0.366(4) [0.3578] | 4.56(36) $\times 10^{-16}$ | 6.05(43) $\times 10^{-6}$ |
| 2D saturated RSA ($N \approx 10^7$) | 0.360(4) [0.3473] | 6.14(54) $\times 10^{-18}$ | 5.93(49) $\times 10^{-6}$ |
| 3D saturated RSA ($N \approx 10^3$) | 0.293(10) [0.2633] | 6.03(2) $\times 10^{-8}$ | 5.76(2) $\times 10^{-6}$ |
| 3D saturated RSA ($N \approx 10^4$) | 0.277(7) [0.2436] | 2.91(3) $\times 10^{-9}$ | 5.66(5) $\times 10^{-8}$ |
| 3D saturated RSA ($N \approx 10^5$) | 0.264(6) [0.2477] | 1.39(5) $\times 10^{-10}$ | 5.57(16) $\times 10^{-6}$ |
| 3D saturated RSA ($N \approx 10^6$) | 0.252(7) [0.2374] | 6.44(32) $\times 10^{-12}$ | 5.69(22) $\times 10^{-6}$ |

[a] We note that the saturated packing fractions of RSA in $d = 2$ and 3 are 0.54707 and 0.38413, respectively [2]. The values of $\phi^{(1)}_{\max}$ in the square brackets $[\cdot]$ represent the minimal values that we observed. To compare different spectral densities, both progenitor packings and constructed dispersions are rescaled to the packing fraction $\phi = 0.01$. Values of $\tilde{\chi}_V(k \to k_{\min})$ are computed by averaging spectral densities at the three lowest wavenumbers. The uncertainties are sample standard deviations.

## III. MULTISCALE-DISK TILINGS

Simulation parameters employed to construct multiscale-disk tilings are summarized in Table III. Figure 2 summarizes the number of inserted disks in the $m$th stage, which demonstrates whether the packings become saturated or whether their covering fraction $\eta_m$ is lower than the scheduled one. Specifically, $N_m/N < 1$ in certain stages implies that the procedure fails to insert a desired number of spheres. Then, some stages with $N_m/N > 1$ immediately follow because the algorithm tries to insert more spheres than $N$ to keep up with the scheduled covering fractions.

When $p = 1.5$, saturation hardly occurs so that the covering fraction is virtually identical to the theoretical values. However, the covering fraction increases slowly compared with cases of $p > 1.5$. For $p = 1.6$, saturation often occurs, but the procedure immediately keeps up the scheduled covering fraction. For $p > 1.6$, however, saturation occurs at very early stages, and once saturation occurs $N_m/N$ never becomes unity, i.e., the packings never keep up with the scheduled covering fraction. Saturation often results in significantly slowing-down computation speed. This is because near saturation, the voxel-list algorithm [2] is designed to split voxels increasingly finer, which sometimes can require a huge amount of memory as well as computational time. Therefore, it is desirable to use $p < 2$.

TABLE III. Simulation parameters employed in multiscale-disk tilings

| Scaling exponent $p$ | $N$ | $v_1(D_1/2)$ |
|---|---|---|
| 1.5 | 383 | 0.00099946053 |
| 1.6 | 438 | 0.00099883599 |
| 1.7 | 487 | 0.00099956156 |
| 1.8 | 532 | 0.00099865565 |

[a] A upper bound $v_{\max}/\mathcal{V}_d$ of cell volume is set to be 0.001. For each scaling exponent $p$, we constructed 50 configurations.

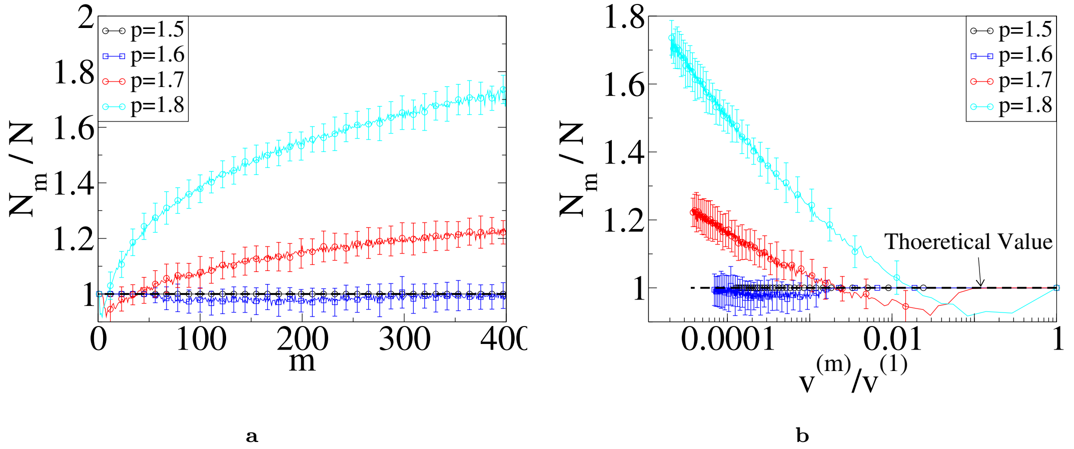


FIG. 2. (a) The number $N_m$ of spheres inserted in the $m$th stage in our multiscale-disk tilings. (b) The inserted number $N_m$ as a function of cell-volumes $v^{(m)}$. Error bars represent sample standard deviations.

* torquato@princeton.edu

[1] C. H. Rycroft, “VORO++: a three-dimensional Voronoi cell library in C++,” Chaos **19**, 041111 (2009).
[2] G. Zhang and S. Torquato, “Precise algorithm to generate random sequential addition of hard hyperspheres at saturation,” Phys. Rev. E **88**, 053312 (2013).
